# Supplementary material for: A Hopfield neural network in magnetic films with natural learning
Source: arXiv:2101.03016 source file (2021-01-08)
Supplement: Supplementary file 1 [file SM_V3.8.pdf]

# Supplemental Materials: A Hopfield neural network in magnetic films with natural learning

Weichao Yu (余伟超),[1] Jiang Xiao (萧江),[2,3,4,*] and Gerrit E. W. Bauer (包格瑞)[5,1,6]

[1]*Institute for Materials Research, Tohoku University, Sendai 980-8577, Japan*
[2]*Department of Physics and State Key Laboratory of Surface Physics, Fudan University, Shanghai 200433, China*
[3]*Institute for Nanoelectronics Devices and Quantum Computing, Fudan University, Shanghai 200433, China*
[4]*Shanghai Research Center for Quantum Sciences, Shanghai 201315, China*
[5]*WPI-AIMR, Tohoku University, Sendai 980-8577, Japan*
[6]*Zernike Institute for Advanced Materials, Groningen University, Netherlands*

## CONTENTS

I. Numerical Method 2

II. Conductance Matrix 3

III. Inferring Process 3

IV. Planar and Anomalous Hall Effects 4

V. Disorder 5

VI. Spin-Transfer Torque 6

VII. Interfacial DMI 7

References 10

* xiaojiang@fudan.edu.cn

## I. NUMERICAL METHOD

We simulate dynamics of current-driven magnetic textures by solving Eqs. (1, 4) self-consistently using COMSOL Multiphysics [1], complemented by the AC/DC module and a homemade module for micromagnetics. The right and left edges of the square sample are connected to high mobility metallic electrodes at constant potentials. All other boundaries satisfy the zero-flow condition $\mathbf{n} \cdot \mathbf{j} = 0$ for the electric current, where $\mathbf{n}$ is the surface normal. Fig. S1(c) proves that the calculations conserve charge since $\nabla \cdot \mathbf{j} = 0$. The curl $(\nabla \times \mathbf{j})_z$ in Fig. S1(d) identifies current vortices and Oersted magnetic fields. The total electric current $I = -\int \mathbf{n} \cdot \mathbf{j}\, dS$ through a surface $S$.

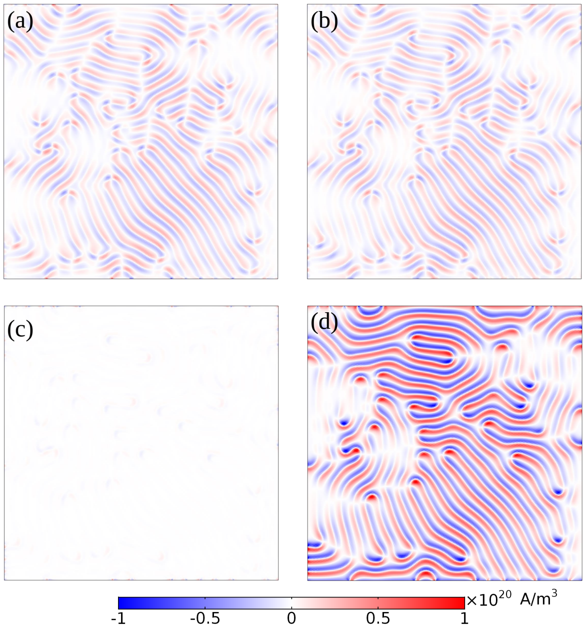


Figure S1. Spatial derivatives of electric current for the texture of Fig. 1(a) in the main text for a voltage difference $V_0 = 0.02\,\mathrm{V}$ between the left and right edges. (a) $\partial j_x/\partial x$, (b) $\partial j_y/\partial y$, (c) $\nabla \cdot \mathbf{j}$, and (d) $(\nabla \times \mathbf{j})_z = \partial j_y/\partial x - \partial j_x/\partial y$.

The dimensions of the sample in Fig. 1 of the main text are $400\,\mathrm{nm} \times 400\,\mathrm{nm}$. The diameter of the disk in Fig. 2 is $1\,\mu\mathrm{m}$. The diameter of the electrodes is $100\,\mathrm{nm}$ and their distance is $400\,\mathrm{nm}$. The textures are two-dimensional, so the film thickness of $1\,\mu\mathrm{m}$ only affects the conductance. The parameters listed below [2] are typical for materials with chiral textures such as Pt/CoFe/MgO [3] multilayers.

We initialize the texture starting from a uniformly magnetized film in the $z$ direction. The DMI generates a magnetic boundary condition $2A\partial_n \mathbf{m} = D(\mathbf{m} \times \mathbf{n})$ [4], which twists the magnetization at the edges. We then let time evolve under a symmetry-breaking in-plane magnetic field that forces the magnetization to settle into irregular initial configurations. During training, a binary array of voltages $\mathbf{V} = \{V_i\}$ with $V_i = \pm V_0$ and $V_0 = 0.04\,\mathrm{V}$ is maintained on the nodes for more than $100\,\mathrm{ns}$. The

| Name | Parameters | Value | Unit |
|---|---|---|---|
| Exchange constant | $A$ | $1.949 \times 10^{-11}$ | A·m |
| Easy-axis anisotropy | $K$ [a] | $4.872 \times 10^{5}$ | A/m |
| Saturation magnetization | $M_s$ | $4.9 \times 10^{5}$ | A/m |
| Gilbert damping | $\alpha$ | 0.3 | 1 |
| Field-like torque coefficient | $\beta$ | $0 \sim 0.3$ | 1 |
| Gyromagnetic ratio | $\gamma$ | $2.21 \times 10^{5}$ | Hz/(A/m) |
| DMI | $D$ | $6.5 \times 10^{-3}$ | A |
| Isotropic conductivity | $\sigma_0$ [b] | $5 \times 10^{6}$ | S/m |
| Spin polarization | $P$ | 0.6 | 1 |

[a] Half value is used compared to the original reference.
[b] $\sigma_0 = (\sigma_{\parallel} + 2\sigma_{\perp})/3$.

Table I. Parameter values

inferring voltages are small enough to not to affect the texture.

## II. CONDUCTANCE MATRIX

The quantity of central interest are the matrix elements of the conductance matrix $G_{ij}$ Eqs. (5,6) for an arbitrary magnetization configuration. The current-voltage relation of four contacts

$$\begin{pmatrix} I_1 \\ I_2 \\ I_3 \\ I_4 \end{pmatrix} = \begin{pmatrix} G_{11} & G_{12} & G_{13} & G_{14} \\ G_{21} & G_{22} & G_{23} & G_{24} \\ G_{31} & G_{32} & G_{33} & G_{34} \\ G_{41} & G_{42} & G_{43} & G_{44} \end{pmatrix} \begin{pmatrix} V_1 \\ V_2 \\ V_3 \\ V_4 \end{pmatrix}. \tag{S1}$$

is governed by Kirchhoff's law. By setting the voltage on $k$-th node $V_k = V_0$ and $V_{j\neq k} = 0$, we retrieve the matrix elements $G_{ik}$ by the current $I_i$ into $i$-th node: $G_{ik} = I_i/V_0$.

We adopt a texture-independent conductance matrix $\hat{G}_0 = \eta\hat{G}_\perp$, where $\hat{G}_\perp$ is the conductance of a perpendicularly (along $\hat{\mathbf{z}}$) magnetized film and the empirical scaling factor $\eta = 0.75$ improves the network performance and may correct for contributions from the anomalous Hall effect (see Secion IV). For our set of parameters, we calculate (in units of Siemens (S))

$$\hat{G}_0 = \begin{pmatrix} +9.9 & -4.3 & -1.2 & -4.3 \\ -4.3 & +9.9 & -4.3 & -1.2 \\ -1.2 & -4.3 & +9.9 & -4.3 \\ -4.3 & -1.2 & -4.3 & +9.9 \end{pmatrix}. \tag{S2}$$

This is a parasitic reference conductance in parallel with a hypothetical system with conductances $G'_{ij}[\mathbf{m}] = G_{ij}[\mathbf{m}] - G^0_{ij}$. The conductance matrices of the trained magnetization configurations in Fig. 2(a-e) are:

$$\hat{G}'_{+-+-} = \begin{pmatrix} +0.9 & -0.7 & +0.1 & -0.3 \\ -0.7 & +1.3 & -0.2 & -0.3 \\ +0.1 & -0.2 & +0.7 & -0.6 \\ -0.3 & -0.3 & -0.6 & +1.2 \end{pmatrix}, \tag{S3}$$

$$\hat{G}'_{+--+} = \begin{pmatrix} -0.5 & +0.0 & -0.2 & +0.7 \\ +0.0 & -0.8 & +0.7 & +0.0 \\ -0.2 & +0.7 & +0.4 & -0.9 \\ +0.7 & +0.0 & -0.9 & +0.2 \end{pmatrix}, \tag{S4}$$

$$\hat{G}'_{++-+} = \begin{pmatrix} +0.0 & +0.0 & -0.2 & +0.2 \\ +0.0 & +0.6 & -0.7 & +0.1 \\ -0.2 & -0.7 & +1.4 & -0.5 \\ +0.2 & +0.1 & -0.5 & +0.3 \end{pmatrix}. \tag{S5}$$

The non-diagonal elements $G'_{ij}$ become more negative ($|G'_{ij}|$ increases) when $V_i \neq V_j$, but $G'_{ij}$ between nodes with same voltages ($V_i = V_j$) may either increase or decrease by the non-local competition with other connections.

## III. INFERRING PROCESS

The patterns stored in the trained Hopfield network can be inferred (read-out) by searching for the minima of the energy function in the space of the binary voltage inputs using standard algorithms. We illustrate the process here by a synchronous or asynchronous iterative process and statistical simulated annealing [5].

Synchronous updating involves all neurons simultaneously, starting from an arbitrary guess initial state $\{V_i(t=0)\}$. The values of all neurons (voltage on each electrode) at time $t+1$ are updated as $V_i(t+1) = \mathrm{sign}(I'_i(t))V_0$, where $I'_i(t) = G'_{ij}V_j(t)$ is the reduced current Eq. (6). After several iterations, the network reaches a the fixed point with $V_i(t+1) = V_i(t)$, which represents the local minimum of the objective function or energy Eq. (7). In the asynchronous process, only one neuron is updated at each time step, chosen either randomly or in a fixed sequence.

Both methods are deterministic and may end up in a local rather than the global minimum. In stochastic annealing, the network becomes a Boltzmann machine with the same energy function Eq. (7) [5]. The reversal of the voltage at a randomly chosen

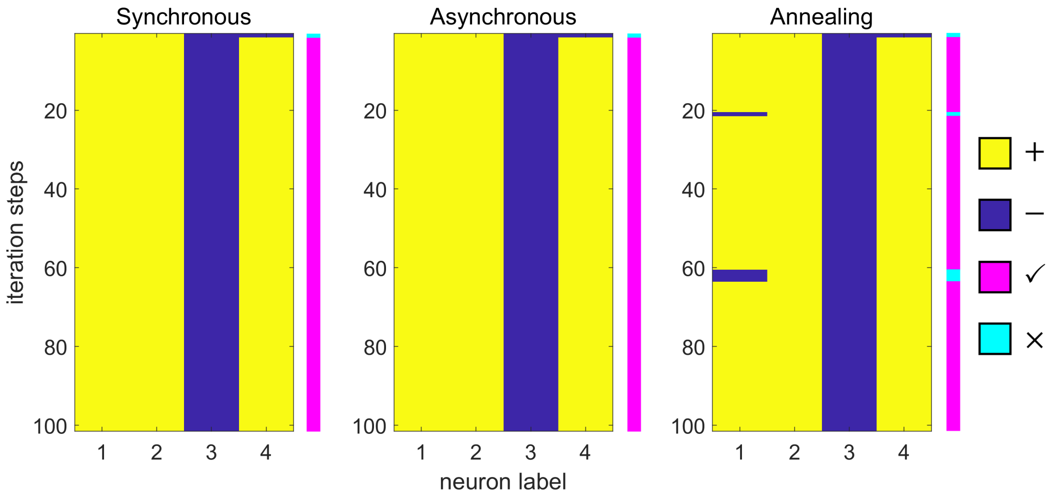


Figure S2. The inferring performance of three methods described in the text. The state of each neuron is represented by "$+$" (yellow) or "$-$" (blue). The initial guess $\{++--\}$ and subsequent ones at each step are compared with the desired one $\{++-+\}$, indicated by the color magenta (cyan) when they agree (disagree). The effective temperature in the annealing process is a constant $T = 10^{-4}$ W.

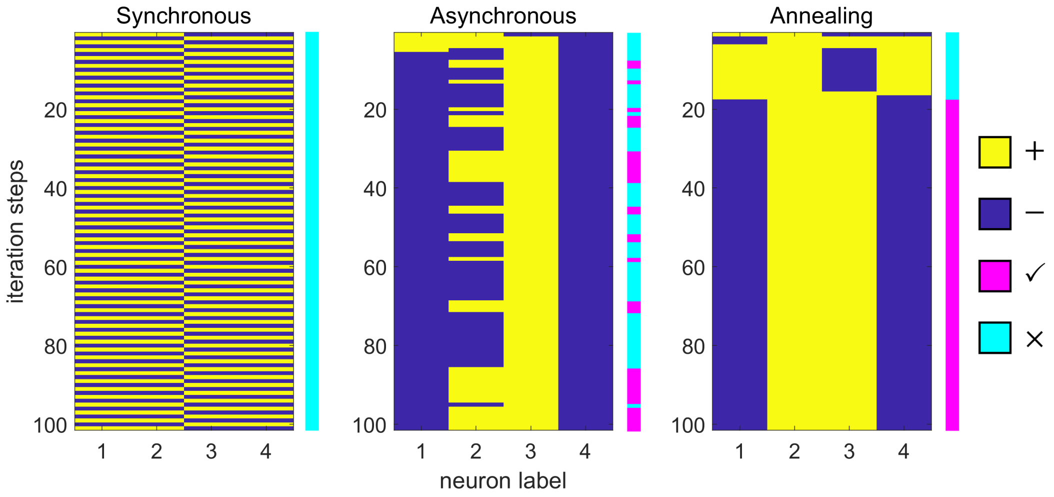


Figure S3. Same as Fig. S2, but for a network trained for $\{+--+\}$.

site during each time step $V_i(t+1) = -V_i(t)$, changes $\Delta E' = E'(t+1) - E'(t)$ and is accepted with Boltzmann probability $p = 1/(1+\exp\{\Delta E'/T\})$ for a temperature $T$ which may be gradually reduced [5].

The simulated inferring results for the pattern stored in Fig. 2(f) $\{++-+\}$ are shown in Fig. S2 for the three methods. Starting with the initial trial state of $\{++--\}$, all methods quickly arrive at the desired state of $\{++-+\}$ or the equivalent $\{--+-\}$. On the other hand, according to Fig. S3, deterministic methods do not converge properly for the pattern stored in Fig. 2(e), while the stochastic annealing performs much better. The reason is the orthogonality of the trained and initial patterns.

## IV. PLANAR AND ANOMALOUS HALL EFFECTS

The planar Hall effect (PHE) is a direct consequence of anisotropic magnetoresistance. In its presence an in-plane applied electric field generates a charge current along $\mathbf{m}(\mathbf{m}\cdot\mathbf{E})$ [6], which has a transverse component unless $\mathbf{E}$ is parallel or normal to $\mathbf{m}$. We assess the PHE by the Hall bar configuration in Fig. S4. The simulation is carried out self-consistently by our COMSOL [1] implementation with micromagnetics and AC/DC modules (including electrical current and circuit interfaces). The planar Hall voltage does not vanish in the presence of maze domains, but is very small ($\sim 0.1\% V_0$).

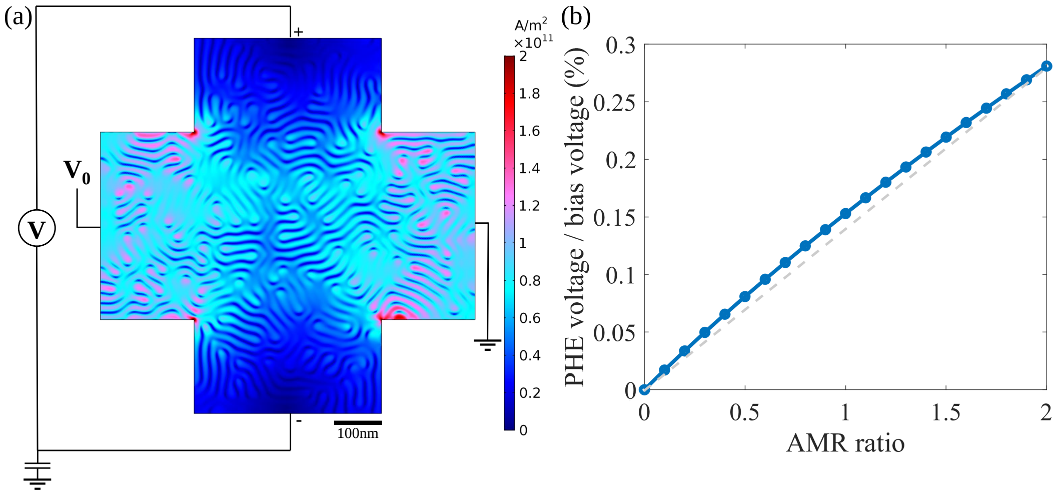


Figure S4. (a) Simulations of the planar Hall effect. A voltage bias $V_0 = 0.02\,\mathrm{V}$ is applied over the left and right edges. The top and bottom edges are connected by a high-impedance voltmeter. (b) PHE signal $V/V_0$ versus the AMR parameter $a$. The dashed straight line is a guide to the eye emphasizing a non-linear dependence of the PHE caused by the charge current distribution dependence on $a$ in a textured magnetic film. Here the anomalous Hall conductivity is set to zero.

In ferromagnetic materials with broken time-reversal symmetry, spin-orbit interaction causes the anomalous Hall effect (AHE) [7]. The AHE current $\sim \mathbf{m}\times\mathbf{E}$ [6], which for an in-plane magnetic field is governed by the perpendicular magnetization. In the presence of maze domains, the positive and negative $z$ components of magnetization cancel to a large extent with $\int m_z(\mathbf{r})d\mathbf{r} \simeq 0$, indicating negligibly small effects. In order to verify this expectation we include AHE terms to the conductivity matrix

$$\Sigma[\mathbf{m}] = \sigma_\perp \mathbb{I} + \sigma_\delta \begin{pmatrix} m_x^2 & m_x m_y \\ m_y m_x & m_y^2 \end{pmatrix} + \sigma_{\mathrm{AHE}} \begin{pmatrix} 0 & m_z \\ -m_z & 0 \end{pmatrix} \tag{S6}$$

where the first two terms are used in main text and the last term is the AHE [7]. The AHE is usually of the same order of magnitude as the AMR [6], so we adopt $\sigma_{\mathrm{AHE}}/\sigma_0 = 1.5$ for consistency, where $\sigma_0$ is the isotropic conductivity as listed in the parameter table.

Starting from the random configuration in Fig. S4(a), a current density $j = 1.4\times 10^{12}\,\mathrm{A/m^2}$ applied in the $x$ direction for $15\,\mathrm{ns}$ leads to the magnetization configuration at time step $t = 20\,\mathrm{ns}$ as shown in Fig. S5(a) with a high conductance state in the $x$ direction. We record the time-dependent transverse voltages in the Hall bar in Fig. S4. The Hall voltage in the presence of (i) only PHE, (ii) only AHE and (iii) both PHE and AHE are shown in Fig. S5(b), indicating low Hall voltage ratios of $\sim \pm 1\%$ as expected. Furthermore, PHE and AHE voltages turn out to cancel to a large extent. Switching off the voltage releases an exchange spring energy at the edges that causes the inertial effects observed after $15\,\mathrm{ns}$. We disregard the small electromotive forces generated by such slow magnetization dynamics.

The net in-plane magnetization is quite rigid under a large chiral DMI, but an applied external magnetic field normal to the film can induce a net significant $z$-component that can be monitored by the AHE. We illustrate this effect by a time-dependent magnetic field $H = 4\times 10^4 t\,\mathrm{A/(m{\cdot}ns)}$ normal to the film applied to the initial configuration in Fig. S4(a). The textures at different times are shown in Fig. S6(a)-(c) and the corresponding PHE and AHE voltages are plotted in (d). With increasing $+z$ component magnetization, the AHE signal increases significantly, while the PHE signal remains to be very small.

## V. DISORDER

Impurities and disorder may reduce the plasticity of the magnetic texture through magnetization pinning and hamper the training efficiency. Here we demonstrate that the performance of the Hopfield network is not severely affected as long as the pinning is not too strong. We model the disorder by an inhomogeneous crystalline anisotropy $K'(\mathbf{r}) = K[1 + 0.5\zeta(\mathbf{r})]$, with $\zeta(\mathbf{r})$ the fluctuation function plotted in Fig. S7(a). Fig. S7 shows that the disorder substantially modulates the magnetization profile from that in Fig. 2. Nevertheless, the clear minima in the trained energy function plotted in Fig. S7(b) indicate that the disorder does not affect the quality of the network.

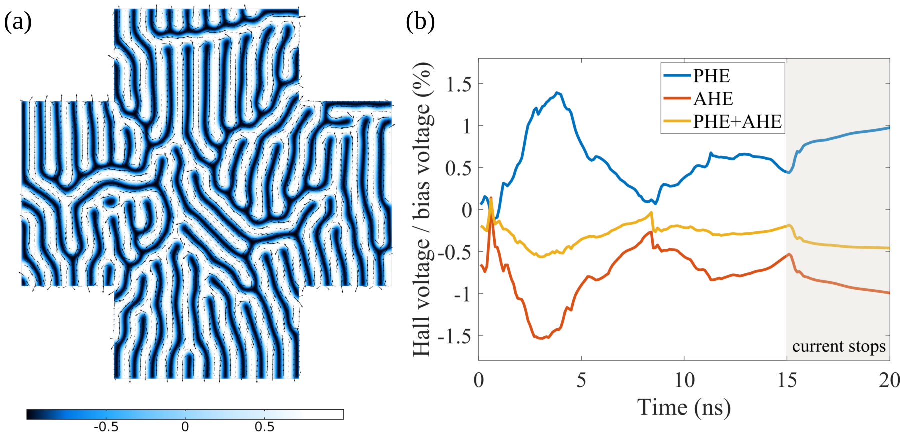


Figure S5. (a) Magnetization configuration at $t$ =20 ns, driven by global spin-transfer torque with current density $j = 1.4 \times 10^{12}$ A/m$^2$ lasting for 15 ns. (b) Hall voltage signal simulated in the presence of (i) only PHE, (ii) only AHE and (iii) both PHE and AHE.

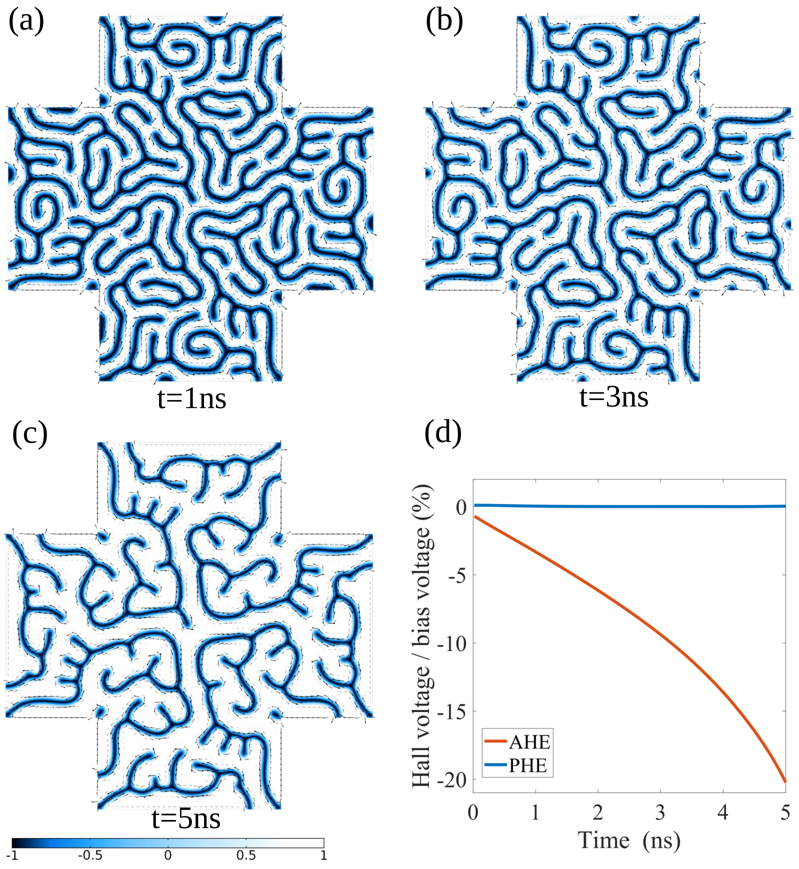


Figure S6. Snapshots of magnetization textures at (a) $t$ =1 ns, (b) $t$ =3 ns and (c) $t$ =5 ns under the external field $H = 4 \times 10^4 t$ A/(m·ns) in $+z$ direction. (d) PHE and AHE voltages.

## VI. SPIN-TRANSFER TORQUE

In the main text, we consider only the damping-like spin-transfer torque Eq. (3), i.e. $\boldsymbol{\tau}_\mathrm{d} = (\mathbf{u} \cdot \nabla)\mathbf{m}$ with $\mathbf{u} \propto \mathbf{j}$. The three torque components at $t = 20$ ns for the current distribution (under voltage vias $V_0 = 0.02$ V) are plotted in Fig. S8. In the steady state, the torque in the $x$ direction ($\tau_x$) is vanishingly small, while the $y$ and $z$ components are compensated by the exchange and anisotropy torques. The AMR enhances the conductance in the current-induced steady state since much of the magnetization is

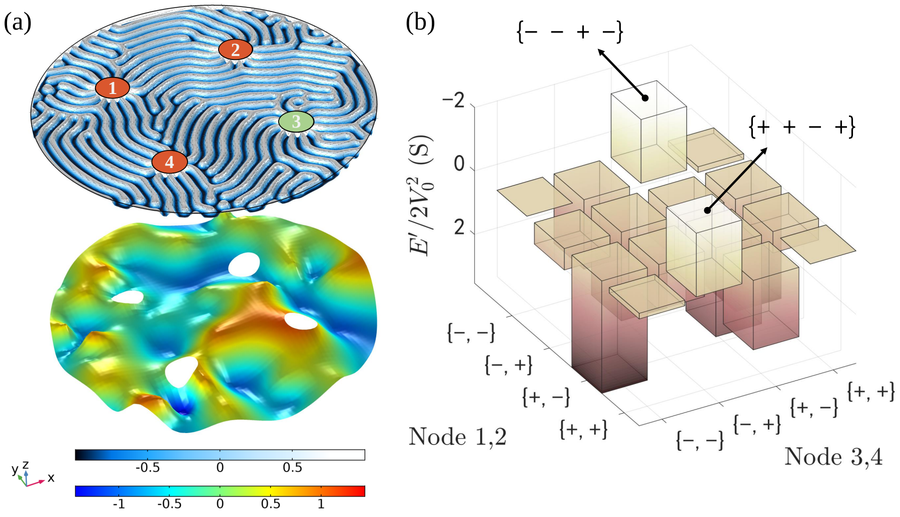


Figure S7. Effect of disorder on a 4-node Hopfield network after training for the state $\{++-+\}$ (Fig. 2(c)(f)). (a) Magnetization distribution (top panel, arrows for in-plane magnetization and color code for out-of-plane magnetization) and fluctuation function $\zeta(\mathbf{r})$ (bottom panel). (b) The energy Eq. (7) calculated under the conditions of Fig. 2.

normal to the current direction, a process that is accelerated by the positive feedback.

In materials with strong spin-orbit coupling, the field-like spin-transfer torque [8] $\boldsymbol{\tau}_{\mathrm{f}} = -\beta \mathbf{m} \times (\mathbf{u} \cdot \nabla)\, \mathbf{m}$ becomes important and competes with the damping-like torque. Fig. S9 shows the texture evolution (from the same configuration as in Fig. 1(a)) under both a damping and a field-like torque with $\beta = 0.1$ and $0.3$. For $\beta = 0.3$ the conductance decreases with time, thereby causing a negative feedback. As explained in the text, a dominantly field-like torque can still drive an efficient network, but an equal amount of field-like and damping-like torques could be detrimental.

## VII. INTERFACIAL DMI

The DMI considered in the main text exists in bulk magnetic materials with broken inversion symmetry. Surfaces and interfaces always break inversion symmetry and cause interfacial/surface DMI in magnetic films and multilayers [9] of the type [4]

$$\mathbf{H}_{\mathrm{intD}} = D\left[(\nabla \cdot \mathbf{m})\hat{\mathbf{z}} - \nabla m_z)\right], \tag{S7}$$

where $\hat{\mathbf{z}}$ is the surface normal. The (otherwise free) magnetic boundary condition at the edges with normal $\mathbf{n}$ then reads

$$\frac{\partial \mathbf{m}}{\partial \mathbf{n}} = \frac{D}{2A}(\hat{\mathbf{z}} \times \mathbf{n}) \times \mathbf{m}. \tag{S8}$$

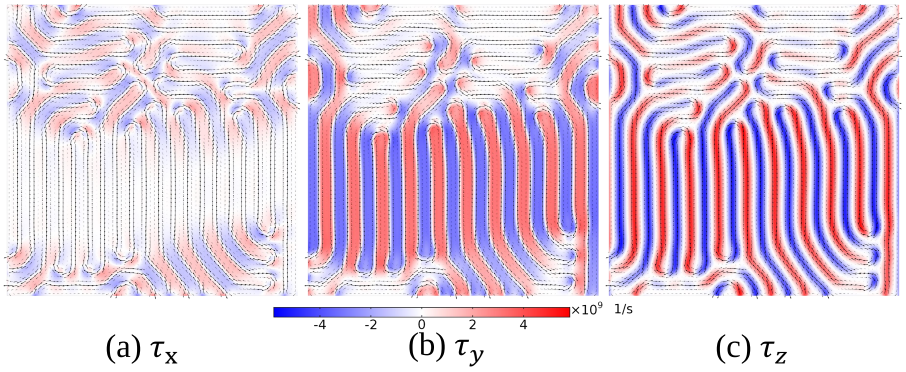


Figure S8. Components of damping-like spin-transfer torque at $t = 20\,\mathrm{ns}$ driving by voltage bias $V_0 = 0.02\,\mathrm{V}$.

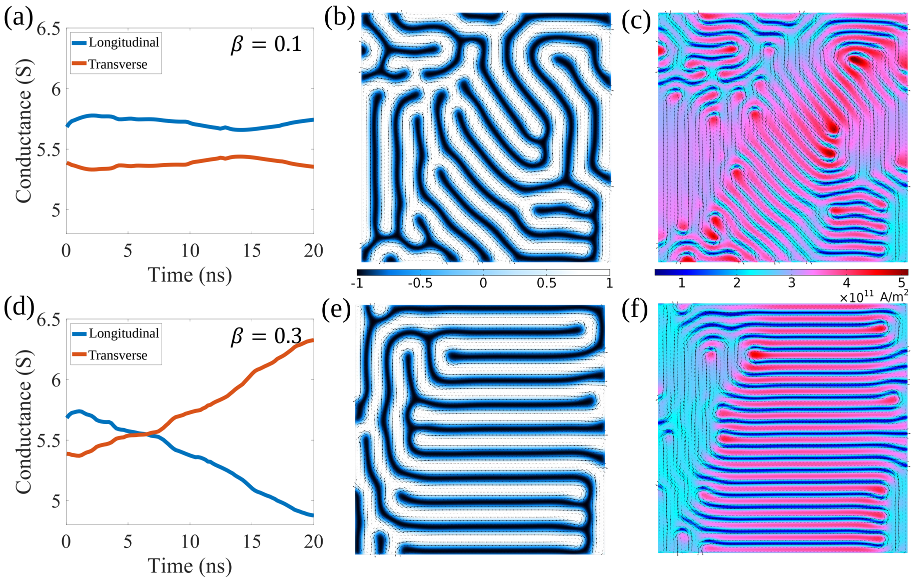


Figure S9. Time evolution of conductance (a, d), magnetization distribution (b, e) and current density distribution (c, f) in the presence of both damping-like torque and field-like torque with $\beta = 0.1$ (a-c) and $\beta = 0.3$ (d-f). The driving voltage $V_0 = 0.02\,\mathrm{V}$. Bulk-type DMI is considered, same as in the main text.

Interfacial DMI favors Néel type rather than Bloch domain walls. Fig. S10 shows the current driven texture evolution, where we also consider the effect of the field-like torque (as discussed in the previous sections) by comparing $\beta = 0$ (left) with $\beta = 0.3$ (right). Fig. S11 shows the corresponding conductance change for the two cases in Fig. S10. The evolution of the magnetic texture and the corresponding conductance behave in an opposite fashion in comparison with the case of bulk DMI, *i.e.*, the longitudinal conductance decreases for $\beta = 0$ (negative feedback), while increases for $\beta = 0.3$ (positive feedback).

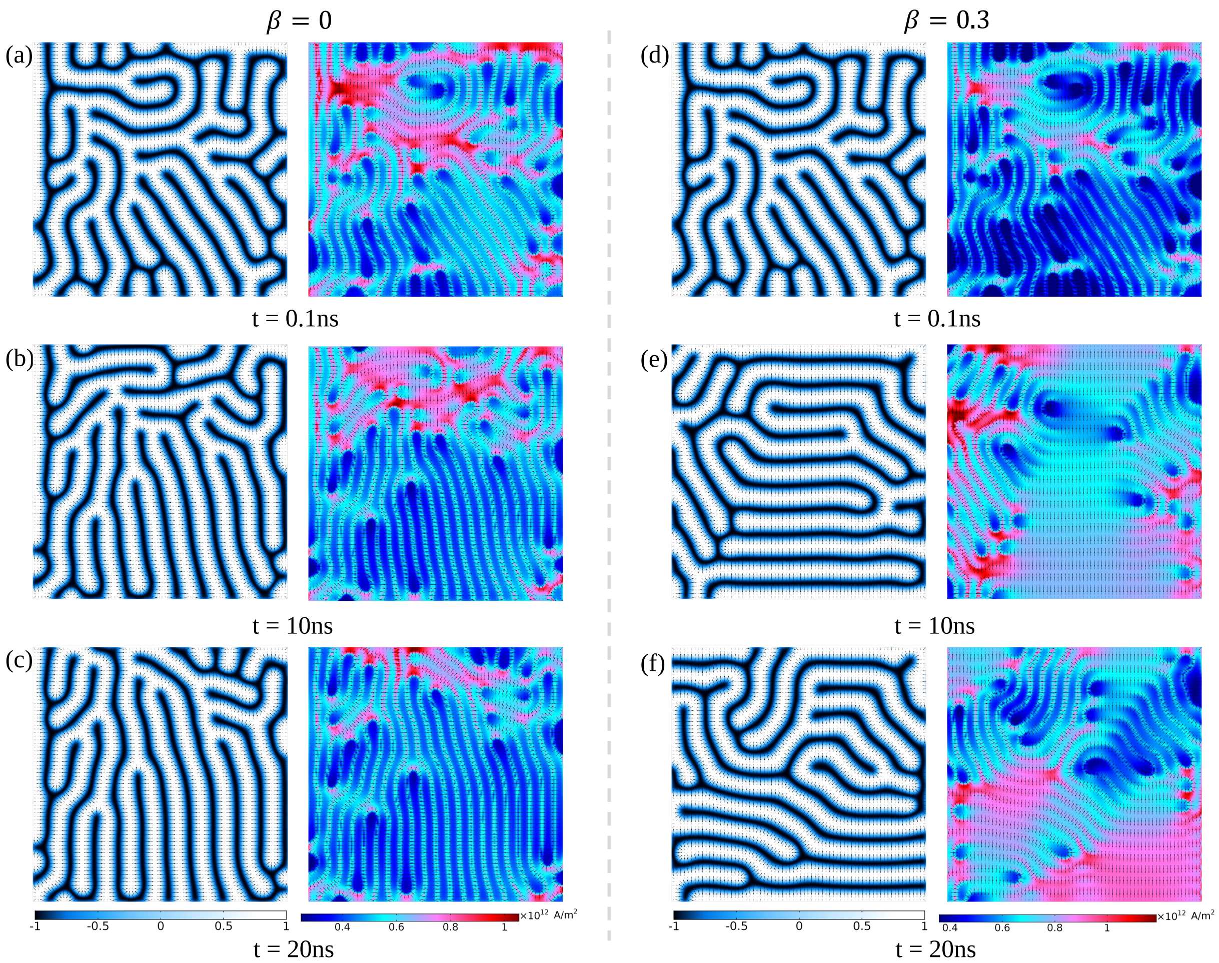


Figure S10. Snapshots of magnetization configuration (left panel) and current density distribution (right panel) at time (a)(d) $t = 0.1\,\text{ns}$, (b)(e) $t = 10\,\text{ns}$ and (c)(f) $t = 20\,\text{ns}$. Voltage difference $V = 0.05\,\text{V}$ is applied on the left and right edges. The electric current induces both damping-like torque and field-like torque with $\beta = 0$ for (a)-(c) and $\beta = 0.3$ for (d)-(f). The DMI Eq.(S7) is here interfacial.

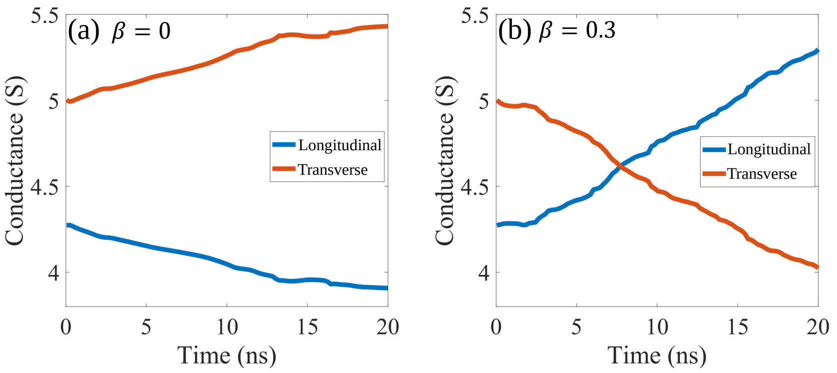


Figure S11. Change of longitudinal (blue) and transverse (red) conductance for the magnetic texture evolution in Fig. S.4. (a) $\beta = 0$ and (b) $\beta = 0.3$.

[1] "COMSOL Multiphysics® v. 5.4. www.comsol.com. COMSOL AB, Stockholm, Sweden." .
[2] D. Prychynenko, M. Sitte, K. Litzius, B. Krüger, G. Bourianoff, M. Kläui, J. Sinova, and K. Everschor-Sitte, Physical Review Applied **9**, 014034 (2018).
[3] S. Woo, K. Litzius, B. Krüger, M.-Y. Im, L. Caretta, K. Richter, M. Mann, A. Krone, R. M. Reeve, M. Weigand, P. Agrawal, I. Lemesh, M.-A. Mawass, P. Fischer, M. Kläui, and G. S. D. Beach, Nature Materials **15**, 501 (2016).
[4] S. Rohart and A. Thiaville, Physical Review B **88**, 184422 (2013).
[5] R. Rojas, *Neural Networks: A Systematic Introduction* (Springer Science & Business Media, 2013) google-Books-ID: 4rESBwAAQBAJ.
[6] T. Taniguchi, J. Grollier, and M. Stiles, Physical Review Applied **3**, 044001 (2015), publisher: American Physical Society.
[7] N. Nagaosa, J. Sinova, S. Onoda, A. H. MacDonald, and N. P. Ong, Reviews of Modern Physics **82**, 1539 (2010), publisher: American Physical Society.
[8] S.-M. Seo, K.-J. Lee, H. Yang, and T. Ono, Physical Review Letters **102**, 147202 (2009).
[9] A. Fert, V. Cros, and J. Sampaio, "Skyrmions on the track," (2013).
